# Supplementary material for: Obfuscation of Pseudo-Deterministic Quantum Circuits
Source: arXiv:2302.11083 source file (2023-11-19)
Supplement: Supplementary file 1 [file appendix-predicate.tex]

\section{Remaining Proofs from \cref{subsec:com-def}}\label{sec:appendix-predicate}

In this appendix, we prove the following lemma.

\begin{lemma}
Any Pauli functional commitment that satisfies \emph{single-bit binding with public decodability} with security $p(\secp) = \poly(\secp)$ also satisfies $m$-bit \emph{predicate binding with public decodability} for any $m$ such that $m \leq p/4$.
\end{lemma}

\begin{proof}
Suppose that the commitment does not satisfy $m$-bit predicate binding with public decodability, so there exist incompatible predicates $(W_0, W_1)$ and an adversary $(\sC_\secp, \sU_\secp)$ such that 

\begin{align*}
    \Pr\left[\bigg\|\Pi_{\bdk,\bc,W_1}\sU_\secp^{\bCK,\DecZ[\bdk]}\Pi_{\bdk,\bc,W_0}\ket{\psi}\bigg\| \geq \nonnegl(\secp)\right] \geq \nonnegl(\secp),
\end{align*}

where the probability is over

\begin{align*}
    &\{\dk_i,\ket{\ck_i},\cCK_i \gets \Gen(1^\secp)\}_{i \in [m]}, \\
    &(\ket{\psi},\bc) \gets \sC_\secp^{\bCK,\DecZ[\bdk],\DecX[\bdk]}(\ket{\mathbf{\bck}}).
\end{align*}

%\begin{align*}\Pr_{\{\dk_i,\ket{\ck_i},\cCK_i \gets \Gen(1^\secp)\}_{i \in [m]}}&\left[\bigg\|\Pi_{\bdk,\bc,W_1}\cU_\secp^{\cCK,\DecZ[\bdk]}\Pi_{\bdk,\bc,W_0}\ket{\psi}\bigg\| \geq \nonnegl(\secp) : (\ket{\psi},\bc) \gets \cC_\secp^{\cCK,\DecZ[\bdk],\DecX[\bdk]}(\ket{\mathbf{\bck}})\right]  \\ & \geq \nonnegl(\secp). \end{align*}

Observe that for any $\bCK, \bdk, \bc,$ and $\ket{\psi}$, 

\begin{align*}
    &\bigg\|\Pi_{\bdk,\bc,W_1}\sU_\secp^{\bCK,\DecZ[\bdk]}\Pi_{\bdk,\bc,W_0}\ket{\psi}\bigg\| \\ 
    &= \bigg\|\left(\sum_{w_1 \in W_1} \bigotimes_{i: w_{1,i} \neq *}\Pi_{\dk_i,c_i,w_{1,i}} \right) \sU_\secp^{\bCK,\DecZ[\bdk]} \left(\sum_{w_0 \in W_0} \bigotimes_{i: w_{0,i} \neq *}\Pi_{\dk_i,c_i,w_{0,i}} \right) \ket{\psi}\bigg\| \\
    &= \bigg\|\sum_{w_1 \in W_1, w_0 \in W_0} \left(\bigotimes_{i: w_{1,i} \neq *}\Pi_{\dk_i,c_i,w_{1,i}}\right) \sU_\secp^{\bCK,\DecZ[\bdk]} \left(\bigotimes_{i: w_{0,i} \neq *}\Pi_{\dk_i,c_i,w_{0,i}}\right) \ket{\psi} \bigg\| \\ 
    &\leq \sum_{w_1 \in W_1, w_0 \in W_0}\bigg\| \left(\bigotimes_{i: w_{1,i} \neq *}\Pi_{\dk_i,c_i,w_{1,i}}\right) \sU_\secp^{\bCK,\DecZ[\bdk]} \left(\bigotimes_{i: w_{0,i} \neq *}\Pi_{\dk_i,c_i,w_{0,i}}\right) \ket{\psi} \bigg\| \\ 
    &\leq 3^{2m} \max_{w_1,w_0} \bigg\| \left(\bigotimes_{i: w_{1,i} \neq *}\Pi_{\dk_i,c_i,w_{1,i}}\right) \sU_\secp^{\bCK,\DecZ[\bdk]} \left(\bigotimes_{i: w_{0,i} \neq *}\Pi_{\dk_i,c_i,w_{0,i}}\right) \ket{\psi} \bigg\| \\ 
    &\leq 3^{2m} \max_{w_1,w_0} \bigg\| \Pi_{\dk_i,c_i,1-b} \sU_\secp^{\bCK,\DecZ[\bdk]} \Pi_{\dk_i,c_i,b} \ket{\psi} \bigg\|
\end{align*}

for some $(i,b)$ such that $w_{0,i}=b$ and $w_{1,i}=1-b$ , which are always guaranteed to exist by the fact that $W_1$ and $W_0$ are incompatible predicates.

%\takashi{I think it may be better to clarify what are the output of $\widetilde{\cC}_\secp$. I think the first output $\ket{\psi}$ should also contain $i$ (because otherwise $\widetilde{\cU}_\secp$ cannot know $i$) and so this is actually different from that of $\cC_\secp$. The second output should be $y_i$ where $\by=(y_1,...,y_m)$ is that of $\cC_\secp$.}

Now, consider an adversary $(\widetilde{\sC}_\secp, \widetilde{\sU}_\secp)$ defined as follows. 

\begin{itemize}
    \item $\widetilde{\sC}_\secp$ takes as input a single commitment key $\ket{\ck}$, samples $i \gets [m]$, sets $\ket{\ck_i} \coloneqq \ket{\ck}$, samples $\{\dk_j, \ket{\ck_j},\cCK_j \gets \Gen(1^\secp)\}_{j \in [m] \setminus \{i\}}$, and then runs $\sC_\secp$ until it outputs $\ket{\psi}$ and $\bc$, responding to $\cCK_i,\DecZ[\dk_i],$ and $\DecX[\dk_i]$ queries by using an external oracle, and $\cCK_j,\DecZ[\dk_j],$ and $\DecX[\dk_j]$ queries for $j \neq i$ internally. Finally, $\widetilde{\sC}_\secp$ outputs $\ket{\widetilde{\psi}} \coloneqq (\ket{\psi},\bc,i,\{\dk_j,\cCK_j\}_{j \in [m] \setminus \{i\}})$, and $\widetilde{c} \coloneqq c_i$ where $\bc = (c_1,\dots,c_m)$.
    \item $\widetilde{\sU}_\secp$ is the same as $\sU_\secp$, except that $\cCK_i$ and $\DecZ[\dk_i]$ queries are answered by using an external oracle and $\cCK_j$ and $\DecZ[\dk_j]$ queries for $j \neq i$ are answered internally, using the information passed by $\widetilde{\sC}_\secp$.
\end{itemize}

Then, 

\begin{align*}
    \Pr\left[\bigg\| \Pi_{\dk,\widetilde{c},1-b} \widetilde{\sU}_\secp^{\cCK,\DecZ[\dk]}\Pi_{\dk,\widetilde{c},b}\ket{\widetilde{\psi}}\bigg\| \geq \frac{1}{3^{2m}} \cdot \nonnegl(\secp)\right] \geq \frac{1}{2m} \cdot \nonnegl(\secp),
\end{align*}

where the probability is over

\begin{align*}
    &b \gets \{0,1\},\\
    &\dk,\ket{\ck},\cCK \gets \Gen(1^\secp), \\
    &(\ket{\widetilde{\psi}},\widetilde{y}) \gets \widetilde{\sC}_\secp^{\cCK,\DecZ[\dk],\DecX[\dk]}(\ket{\ck}).
\end{align*}

%\begin{align*}\Pr_{b \gets \{0,1\},\dk,\ket{\ck},\cCK \gets \Gen(1^\secp)}&\left[\bigg\| \Pi_{\dk,\widetilde{c},1-b} \widetilde{\cU}_\secp^{\cCK,\DecZ[\dk]}\Pi_{\dk,\widetilde{c},b}\ket{\widetilde{\psi}}\bigg\| \geq \frac{1}{3^{2m}} \cdot \nonnegl(\secp) : (\ket{\widetilde{\psi}},\widetilde{y}) \gets \widetilde{\cC}_\secp^{\cCK,\DecZ[\dk],\DecX[\dk]}(\ket{\ck})\right] \\ &\geq \frac{1}{2m} \cdot \nonnegl(\secp),\end{align*} 

The $2m$ on the RHS comes from guessing $b \gets \{0,1\}$ (in the description of the experiment), and $\widetilde{\sC}_\secp$ guessing $i \gets [m]$. Since $3^{2m} \cdot \nonnegl(\secp) \leq 2^{4m}$, and $1/2m \cdot \nonnegl(\secp) = \nonnegl(\secp)$, this implies that there must exist some $b \in \{0,1\}$ such that 

\begin{align*}\Pr_{\dk,\ket{\ck},\cCK \gets \Gen(1^\secp)}&\left[\bigg\| \Pi_{\dk,\widetilde{y},1-b} \widetilde{\sU}_\secp^{\cCK,\DecZ[\dk]}\Pi_{\dk,\widetilde{y},b}\ket{\widetilde{\psi}}\bigg\| \geq \frac{1}{2^{4m}} : (\ket{\widetilde{\psi}},\widetilde{y}) \gets \widetilde{\sC}_\secp^{\cCK,\DecZ[\dk],\DecX[\dk]}(\ket{\ck})\right] \geq \nonnegl(\secp),\end{align*}

which means that the commitment does not satisfy single-bit binding with public decodability with security $4m \leq p$, a contradiction.

\end{proof}
