# Supplementary material for: Obfuscation of Pseudo-Deterministic Quantum Circuits
Source: arXiv:2302.11083 source file (2023-11-19)
Supplement: Supplementary file 2 [file appendix-token.tex]

\section{Proofs from \cref{sec:sig-tokens}}\label{sec:appendix-tokens}
